# Supplementary material for: A Mixed-Methods Study of Open-Source Software Maintainers On Vulnerability Management and Platform Security Features
Source: arXiv:2409.07669 source file (2025-02-03)
Supplement: Supplementary file 1 [file appendix.tex]

\appendix

\section{Listing survey questions and outline}\label{sec:surveyqs}

\noindent\textbf{[Study information, eligibility criteria, privacy notice, etc.]}

\vspace{0.2cm}

\noindent\textbf{Eligibility question} Do you reside in an OFAC-sanctioned region or are affiliated with an OFAC-sanction entity?

\vspace{0.2cm}

\noindent\textbf{Main questionnaire:}\vspace{0.1cm}

\noindent1. How do you currently handle vulnerability reports in your OSS project(s)? Please describe in detail.

\vspace{0.1cm}

\noindent2. What tooling or suggested practices, if any, do you use to track and manage vulnerabilities? Please list any software, services, or methodologies you rely on.

\vspace{0.1cm}

\noindent3. How often do you review and update, if necessary, your vulnerability management practices? Please describe in detail.

\vspace{0.1cm}

\noindent4. What are the challenges you currently face in managing OSS vulnerabilities?
Please list all that you can think of.

\vspace{0.1cm}

\noindent5. How would you describe your overall experience(s) with OSS vulnerability management? Please describe in detail.

\vspace{0.1cm}

\noindent6. Which platform security features do you currently have enabled?	Please list all that you have enabled.

\vspace{0.1cm}

\noindent7. What challenges have you faced maintaining or publishing a security policy? Please list all that you can think of.

\vspace{0.1cm}
	
\noindent8. Do you have any suggestions for policies or guidelines that OSS platforms should implement to improve vulnerability management across repositories? If so, please list any policy or guideline recommendations.	

\vspace{0.1cm}

\noindent9. What challenges have you faced maintaining and publishing security advisories? Please list all that you can think of.

\vspace{0.1cm}

\noindent10. What challenges have you faced when considering or using the \textit{Private vulnerability reporting} feature? Please list all that you can think of.

\vspace{0.1cm}

\noindent11. If applicable, please list any alternative mechanisms of reporting (e.g., email) or disclosure you use outside of platform security features. Please list all that you can think of.	

\vspace{0.1cm}

\noindent12. What resources or tools you have found useful for managing vulnerabilities? Please list all that you can think of.

\vspace{0.1cm}

\noindent13. Do you feel that the platform security tools provided by OSS platforms are sufficient for managing vulnerabilities? If not, what additional features or improvements would you like to see?	Please describe in detail.

\vspace{0.1cm}

\noindent14. What resources or support would be most beneficial for you to improve your vulnerability management practices? Please list all that you can think of.

\vspace{0.2cm}

\noindent\textbf{[Background multiple choice questions (\autoref{tab:participants})]}

\section{Semi-structured interview guide}\label{sec:interviewguide}

\noindent\textbf{0. Project maintainer duties}

\vspace{0.1cm}

\noindent0. Can you tell me about your duties as an open-source project maintainer? 

\vspace{0.2cm}

\noindent\textbf{1. Current vulnerability management practices}

%\leftskip=0.5cm\rightskip=0.5cm

\noindent1. Can you elaborate on your process for handling OSS vulnerabilities? \vspace{0.1cm}

\noindent2. What tools or platforms do you find the most effective for tracking and managing vulnerabilities? \vspace{0.1cm}

\noindent3. Are there any aspects of these tools that you find particularly helpful?\vspace{0.1cm}

\noindent4. What tools or platforms do you find the least effective for tracking and managing vulnerabilities? \vspace{0.1cm}

\noindent5. Are there any features of these tools that you find particularly lacking?\vspace{0.1cm}

\noindent6. How do you decide when to review and update your vulnerability management practices? Can you provide an example of a recent update and what prompted it? \vspace{0.1cm}

\vspace{0.1cm} %\leftskip=0cm\rightskip=0cm 

\noindent\textbf{2. Challenges with vulnerability management} \vspace{0.1cm}

\noindent7. In the survey, you mentioned several challenges in managing vulnerabilities, including [mention responses]. Can you provide more details about the most significant challenge(s)?\vspace{0.1cm}

\noindent8. How have these challenges impacted your project and overall workflow?\vspace{0.1cm}

\noindent9. Are there any particular hurdles you overcame? How?\vspace{0.1cm}

\noindent10. How do these hurdles affect your ability to manage vulnerabilities effectively? Can you provide an example?

\vspace{0.2cm}

\noindent\textbf{3. Challenges with platform security features }\vspace{0.1cm}

\noindent11. In the survey, you mentioned several challenges when using specific platform security features, including [mention responses]. Can you provide more details about the most significant challenge(s)?\vspace{0.1cm}

\noindent12. How have these challenges impacted your project and overall workflow?\vspace{0.1cm}

\noindent13. Are there any particular hurdles you overcame? How?\vspace{0.1cm}

\noindent14. How do these hurdles affect your ability to manage vulnerabilities effectively? Can you provide an example?\vspace{0.1cm}

%What specific issues do you encounter when disclosing vulnerabilities to your users? How do you address these issues, and what improvements do you think could be made?

\vspace{0.1cm}

\noindent\textbf{4. Barriers to adopting platform security features }\vspace{0.1cm}

\noindent15. In the survey, you mentioned several barriers when considering using specific platform security features, including [mention responses]. Can you provide more details about the most significant barrier(s)?\vspace{0.1cm}

\noindent16. I noticed you did not mention using [platform security feature(s)]. Could you elaborate?\vspace{0.1cm}

\noindent17. What do you think would motivate you, if possible, to adopt more platform security features?\vspace{0.1cm}

\vspace{0.1cm}

\noindent\textbf{5. Opportunities for improvement and support }\vspace{0.1cm}

\noindent18. You mentioned needing [resources and support] for vulnerability management. Can you expand on the specific types of support that would be most beneficial?\vspace{0.1cm}

\noindent19. In your opinion, what additional features or improvements should OSS platforms implement to better support vulnerability management?\vspace{0.1cm}

\noindent20. How would these improvements make a difference in your project? Workflow?\vspace{0.1cm}

%Are there any resources or communities you rely on that you think others should know about?

%Can you provide examples of support or tools that would be particularly helpful?

%You mentioned some best practices for managing vulnerabilities. Can you describe a few of these in detail? Why do you think these practices are effective?

%How do you think collaboration with the security community can be improved for better vulnerability management?

%Can you share a significant learning experience you had in managing vulnerabilities for your OSS project(s)?

%How has this experience influenced your current practices?

\noindent21. How would you see emerging technologies, such as large language models, support you?\vspace{0.1cm}

\noindent22. Is there anything else you would like to add about software vulnerability management in your OSS project(s)?

%\pagebreak

%\section{Interview participants}\label{sec:participants}

%\vspace{-0.5cm}
%\begin{figure}[ht]
%  \includegraphics[width=0.98\textwidth]{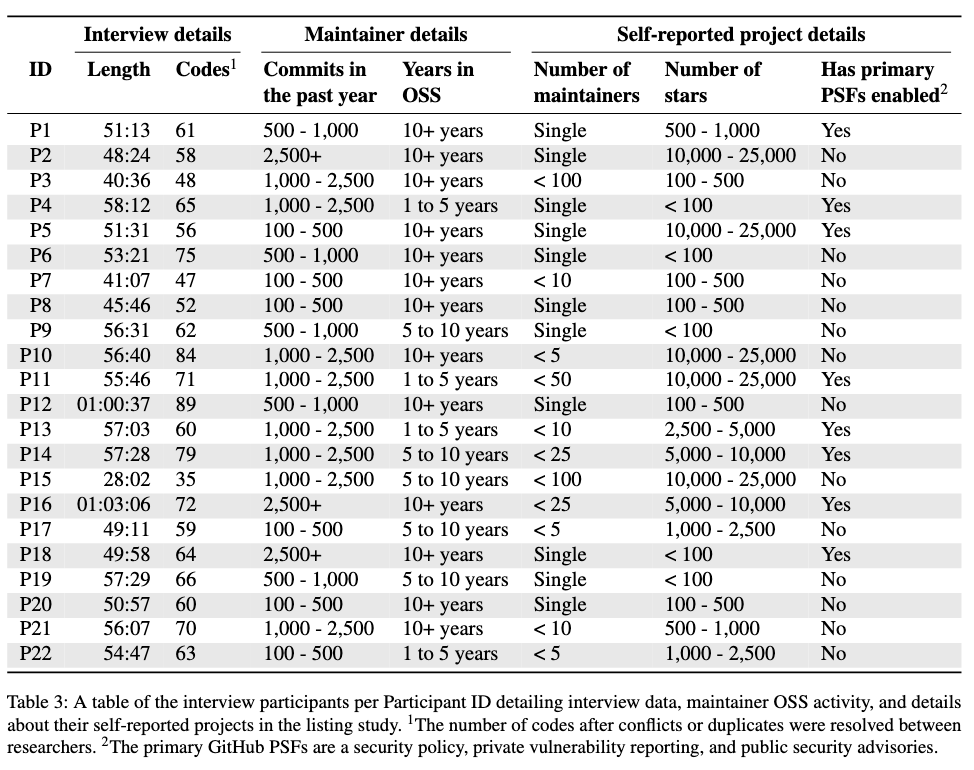}
%\end{figure}
%\clearpage

%\section{Full table of curated codes}\label{sec:fulltable}

%\vspace{-0.2cm}
%\centering
%\begin{figure}[ht!]
%  \includegraphics[width=0.96\textwidth]{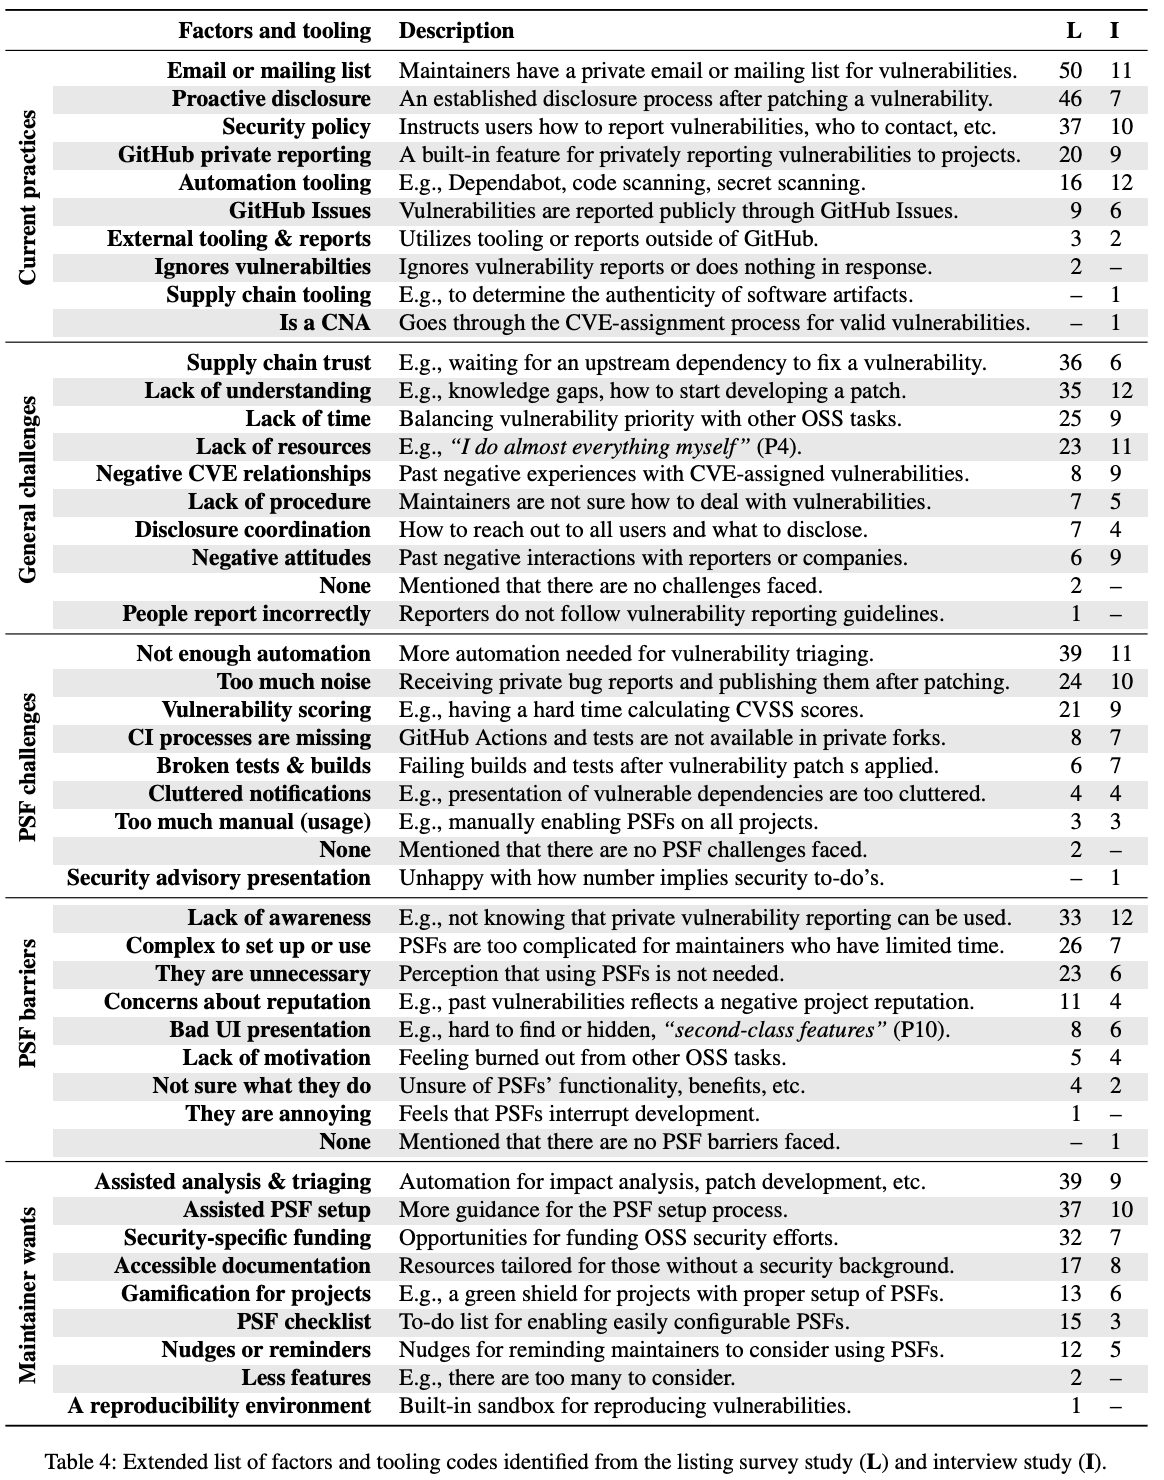}
%\end{figure}
