# Supplementary material for: A Mixed-Methods Study of Open-Source Software Maintainers On Vulnerability Management and Platform Security Features
Source: arXiv:2409.07669 source file (2025-02-03)
Supplement: Supplementary file 2 [file appendix_tables.tex]

\FloatBarrier
 \begin{table*}[h!]
 \centering
 \begin{adjustbox}{width=\textwidth}
 \begin{tabular}{rrllllll}
 \toprule
  & \multicolumn{2}{c}{\textbf{Interview details}} & \multicolumn{2}{c}{\textbf{Maintainer details}} & \multicolumn{3}{c}{\textbf{Self-reported project details}} \\ 
 \cmidrule(lr){2-3} \cmidrule(lr){4-5} \cmidrule(lr){6-8}
 \multicolumn{1}{r}{\textbf{ID}} & \multicolumn{1}{r}{\textbf{Length}} & \multicolumn{1}{l}{\textbf{Codes$^1$}} & \multicolumn{1}{l}{\textbf{Commits in}} & \multicolumn{1}{l}{\textbf{Years in}} & \multicolumn{1}{l}{\textbf{Number of}} & \multicolumn{1}{l}{\textbf{Number of}} & \multicolumn{1}{l}{\textbf{Has primary}} \\
 & & & \multicolumn{1}{l}{\textbf{the past year}} & \multicolumn{1}{l}{\textbf{OSS}} & \multicolumn{1}{l}{\textbf{maintainers}} & \multicolumn{1}{l}{\textbf{stars}} & \multicolumn{1}{l}{\textbf{PSFs enabled$^2$}} \\ 
 \midrule
P1 & 51:13 & 61 & 500 - 1,000 & 10+ years & Single & 500 - 1,000 & Yes \\
\rowcolor{grey1} P2 & 48:24 & 58 & 2,500+ & 10+ years & Single & 10,000 - 25,000 & No \\
P3 & 40:36 & 48 & 1,000 - 2,500 & 10+ years & < 100 & 100 - 500 & No \\
\rowcolor{grey1} P4 & 58:12 & 65 & 1,000 - 2,500 & 1 to 5 years & Single & < 100 & Yes \\
P5 & 51:31 & 56 & 100 - 500 & 10+ years & Single & 10,000 - 25,000 & Yes \\
\rowcolor{grey1} P6 & 53:21 & 75 & 500 - 1,000 & 10+ years & Single & < 100 & No \\
P7 & 41:07 & 47 & 100 - 500 & 10+ years & < 10 & 100 - 500 & No \\
\rowcolor{grey1} P8 & 45:46 & 52 & 100 - 500 & 10+ years & Single & 100 - 500 & No \\
P9 & 56:31 & 62 & 500 - 1,000 & 5 to 10 years & Single & < 100 & No \\
\rowcolor{grey1} P10 & 56:40 & 84 & 1,000 - 2,500 & 10+ years & < 5 & 10,000 - 25,000 & No \\
P11 & 55:46 & 71 & 1,000 - 2,500 & 1 to 5 years & < 50 & 10,000 - 25,000 & Yes \\
\rowcolor{grey1} P12 & 01:00:37 & 89 & 500 - 1,000 & 10+ years & Single & 100 - 500 & No \\
P13 & 57:03 & 60 & 1,000 - 2,500 & 1 to 5 years & < 10 & 2,500 - 5,000 & Yes \\
\rowcolor{grey1} P14 & 57:28 & 79 & 1,000 - 2,500 & 5 to 10 years & < 25 & 5,000 - 10,000 & Yes \\
P15 & 28:02 & 35 & 1,000 - 2,500 & 5 to 10 years & < 100 & 10,000 - 25,000 & No \\
\rowcolor{grey1} P16 & 01:03:06 & 72 & 2,500+ & 10+ years & < 25 & 5,000 - 10,000 & Yes \\
P17 & 49:11 & 59 & 100 - 500 & 5 to 10 years & < 5 & 1,000 - 2,500 & No \\
\rowcolor{grey1} P18 & 49:58 & 64 & 2,500+ & 10+ years & Single & < 100 & Yes \\
P19 & 57:29 & 66 & 500 - 1,000 & 5 to 10 years & Single & < 100 & No \\
\rowcolor{grey1} P20 & 50:57 & 60 & 100 - 500 & 10+ years & Single & 100 - 500 & No \\
P21 & 56:07 & 70 & 1,000 - 2,500 & 10+ years & < 10 & 500 - 1,000 & No \\
\rowcolor{grey1} P22 & 54:47 & 63 & 100 - 500 & 1 to 5 years & < 5 & 1,000 - 2,500 & No \\
   \bottomrule
 \end{tabular}
 \end{adjustbox}
 \caption{A table of the interview participants per Participant ID detailing interview data, maintainer OSS activity, and details about their self-reported projects in the listing study. ${}^{1}$The number of codes after conflicts or duplicates were resolved between researchers. ${}^{2}$The primary GitHub PSFs are a security policy, private vulnerability reporting, and public security advisories.}
    \label{tab:bigasstable2}
 %\end{centering}
 \end{table*}
\FloatBarrier

%\newpage

 \begin{table*}[ht!]
 \centering
 \begin{adjustbox}{width=\textwidth}
 \begin{tabular}{crlrl}
 \toprule
 %\midrule
 & \multicolumn{1}{r}{\textbf{Factors and tooling}} & \multicolumn{1}{l}{\textbf{Description}} & \multicolumn{1}{r}{\textbf{L}} & \multicolumn{1}{l}{\textbf{I}} \\
 \midrule
 \parbox[t]{3mm}{\multirow{10}{*}{\rotatebox[origin=c]{90}{\textbf{Current practices}}}}
   & \textbf{Email or mailing list} & Maintainers have a private email or mailing list for vulnerabilities. & 50 & 11 \\
   & \rowcolor{grey1} \textbf{Proactive disclosure} & An established disclosure process after patching a vulnerability. & 46 & 7 \\
   & \textbf{Security policy} & Instructs users how to report vulnerabilities, who to contact, etc. & 37 & 10 \\
   & \rowcolor{grey1} \textbf{GitHub private reporting} & A built-in feature for privately reporting vulnerabilities to projects. & 20 & 9 \\
   & \textbf{Automation tooling} & E.g., Dependabot, code scanning, secret scanning. & 16 & 12 \\
   & \rowcolor{grey1} \textbf{GitHub Issues} & Vulnerabilities are reported publicly through GitHub Issues. & 9 & 6 \\
   & \textbf{External tooling \& reports} & Utilizes tooling or reports outside of GitHub.  & 3 & 2 \\
   & \rowcolor{grey1} \textbf{Ignores vulnerabilties} & Ignores vulnerability reports or does nothing in response. & 2 & -- \\
   & \textbf{Supply chain tooling} & E.g., to determine the authenticity of software artifacts. & -- & 1 \\
   & \rowcolor{grey1} \textbf{Is a CNA} & Goes through the CVE-assignment process for valid vulnerabilities. & -- & 1 \\
  \midrule
 \parbox[t]{3mm}{\multirow{10}{*}{\rotatebox[origin=c]{90}{\textbf{General challenges}}}}
   & \textbf{Supply chain trust} & E.g., waiting for an upstream dependency to fix a vulnerability. & 36 & 6 \\
   & \rowcolor{grey1} \textbf{Lack of understanding} & E.g., knowledge gaps, how to start developing a patch. & 35 & 12 \\
   & \textbf{Lack of time} & Balancing vulnerability priority with other OSS tasks. & 25 & 9 \\
   & \rowcolor{grey1} \textbf{Lack of resources} & E.g., \textit{``I do almost everything myself''} (P4). & 23 & 11 \\
   & \textbf{Negative CVE relationships} & Past negative experiences with CVE-assigned vulnerabilities. & 8 & 9 \\
   & \rowcolor{grey1} \textbf{Lack of procedure} & Maintainers are not sure how to deal with vulnerabilities. & 7 & 5 \\
   & \textbf{Disclosure coordination} & How to reach out to all users and what to disclose. & 7 & 4 \\
   & \rowcolor{grey1} \textbf{Negative attitudes} & Past negative interactions with reporters or companies. & 6 & 9 \\
   & \textbf{None} & Mentioned that there are no challenges faced. & 2 & -- \\
   & \rowcolor{grey1} \textbf{People report incorrectly} & Reporters do not follow vulnerability reporting guidelines. & 1 & -- \\
 \midrule
   \parbox[t]{3mm}{\multirow{9}{*}{\rotatebox[origin=c]{90}{\textbf{PSF challenges}}}}
   & \textbf{Not enough automation} & More automation needed for vulnerability triaging. & 39 & 11 \\
   & \rowcolor{grey1} \textbf{Too much noise} & Receiving private bug reports and publishing them after patching. & 24 & 10 \\
   & \textbf{Vulnerability scoring} & E.g., having a hard time calculating CVSS scores. & 21 & 9 \\
   & \rowcolor{grey1} \textbf{CI processes are missing} & GitHub Actions and tests are not available in private forks. & 8 & 7 \\
   & \textbf{Broken tests \& builds} & Failing builds and tests after vulnerability patch s applied. & 6 & 7 \\
   & \rowcolor{grey1} \textbf{Cluttered notifications} & E.g., presentation of vulnerable dependencies are too cluttered. & 4 & 4 \\
   & \textbf{Too much manual (usage)} & E.g., manually enabling PSFs on all projects. & 3 & 3 \\
   & \rowcolor{grey1} \textbf{None} & Mentioned that there are no PSF challenges faced. & 2 & -- \\
   & \textbf{Security advisory presentation} & Unhappy with how number implies security to-do's. & -- & 1 \\
  \midrule
   \parbox[t]{3mm}{\multirow{9}{*}{\rotatebox[origin=c]{90}{\textbf{PSF barriers}}}}
   & \rowcolor{grey1} \textbf{Lack of awareness} & E.g., not knowing that private vulnerability reporting can be used. & 33 & 12 \\
   & \textbf{Complex to set up or use} & PSFs are too complicated for maintainers who have limited time. & 26 & 7 \\
   & \rowcolor{grey1} \textbf{They are unnecessary} & Perception that using PSFs is not needed. & 23 & 6 \\
   & \textbf{Concerns about reputation} & E.g., past vulnerabilities reflects a negative project reputation. & 11 & 4 \\
   & \rowcolor{grey1} \textbf{Bad UI presentation} & E.g., hard to find or hidden, \textit{``second-class features''} (P10). & 8 & 6 \\
   & \textbf{Lack of motivation} & Feeling burned out from other OSS tasks. & 5 & 4 \\
   & \rowcolor{grey1} \textbf{Not sure what they do} & Unsure of PSFs' functionality, benefits, etc. & 4 & 2 \\
   & \textbf{They are annoying} & Feels that PSFs interrupt development. & 1 & -- \\
   & \rowcolor{grey1} \textbf{None} & Mentioned that there are no PSF barriers faced. & -- & 1 \\
  \midrule
   \parbox[t]{3mm}{\multirow{9}{*}{\rotatebox[origin=c]{90}{\textbf{Maintainer wants}}}}
   & \textbf{Assisted analysis \& triaging} & Automation for impact analysis, patch development, etc. & 39 & 9 \\   
   & \rowcolor{grey1} \textbf{Assisted PSF setup} & More guidance for the PSF setup process. & 37 & 10 \\
   & \textbf{Security-specific funding} & Opportunities for funding OSS security efforts. & 32 & 7 \\
   & \rowcolor{grey1} \textbf{Accessible documentation} & Resources tailored for those without a security background. & 17 & 8 \\
%   & \textbf{Tooling recommendations} & The ability to provide feedback and make report adjustments. & & &  \\
   & \textbf{Gamification for projects} & E.g., a green shield for projects with proper setup of PSFs. & 13 & 6 \\
   & \rowcolor{grey1} \textbf{PSF checklist} & To-do list for enabling easily configurable PSFs. & 15 & 3 \\   
   & \textbf{Nudges or reminders} & Nudges for reminding maintainers to consider using PSFs. & 12 & 5 \\
   & \rowcolor{grey1} \textbf{Less features} & E.g., there are too many to consider. & 2 & -- \\
   & \textbf{A reproducibility environment} & Built-in sandbox for reproducing vulnerabilities. & 1 & -- \\
%   & \rowcolor{grey1} \textbf{Dependency inspection} & Comments and messaging are available during the review process. &  & &  \\
%   & \rowcolor{grey1} \textbf{Auto-merge configurations} & Streamlined and assisted process of creating CVEs. & & &  \\
  \bottomrule
 \end{tabular}
 \end{adjustbox}
 \caption{Extended list of factors and tooling codes identified from the listing survey study (\textbf{L}) and interview study (\textbf{I}).}
 %\end{centering}
 \end{table*}
